# Supplementary material for: VEMamba: Efficient Isotropic Reconstruction of Volume Electron Microscopy with Axial-Lateral Consistent Mamba
Source: arXiv:2603.00887 source file (2026-07-27)
Supplement: Supplementary file 2 [file X_suppl.tex]

\clearpage
\setcounter{page}{1}
\maketitlesupplementary

\section{MoCo}

\section{EPFL}

\section{CREMI}
